# Supplementary material for: 3D-aware Blending with Generative NeRFs
Source: arXiv:2302.06608 source file (2023-08-16)

Original

Reference

Blend

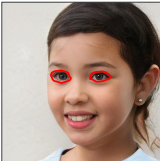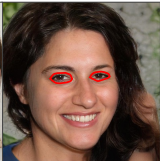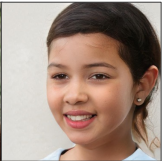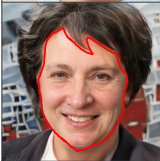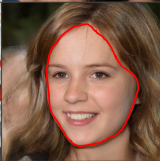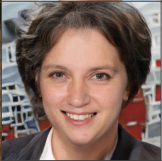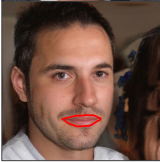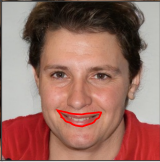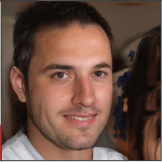

Original

Reference

Blend

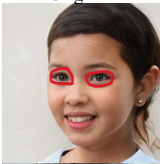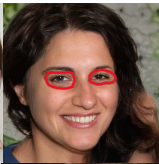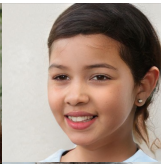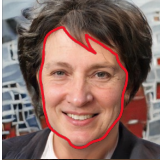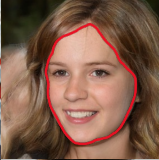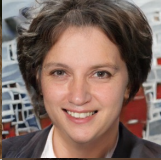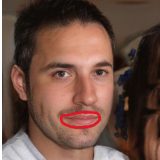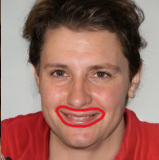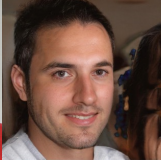

Original

Reference

Blend

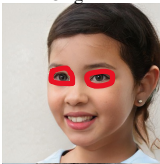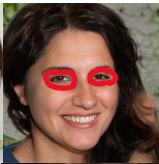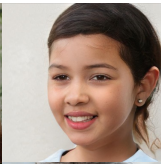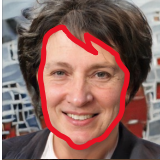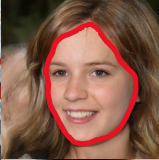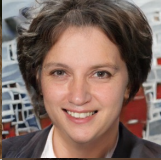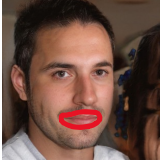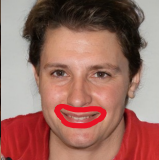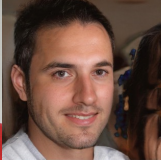

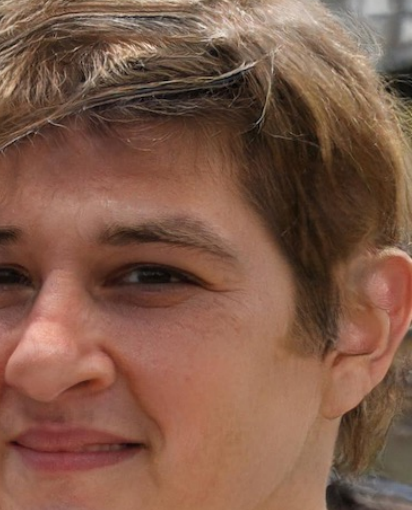

Supplement: Supplementary file 1 [file stylesdf_blend.pdf]
